# Supplementary material for: Adaptive atomic basis sets
Source: arXiv:2404.16942 source file (2024-04-25)
Supplement: Supplementary file 1 [file SI.tex]

\section{Appendix}
\label{Sec:Appendix}

\subsection{Analysis of scaling factors}
As previously discussed, %in Sec. \ref{sec:Results}
our scaling factors $\zeta$ are highly local quantities and depend on the direct chemical environment and closest bonds.
Fig. \ref{fig:Violins} shows the STO-3G scaling factor distribution for each element sorted by the closest bonding partner.
All distributions exhibit spikes at multiple scaling factors, however the optimal values tend to increase (decrease) in the presence (absence) of highly electronegative bonding partners.
Upon examination of some of the molecules, this could be confirmed and $\zeta$ generally appears to be a linked to the local electron density.
As can be seen in Fig. \ref{fig:example_factors}, Carbon for instance has the largest scaling factor in the CF$_4$ molecule ($\zeta_\text{max}=1.19$), while a very small $\zeta$ is found in the negatively charged and triple bonded Carbon atom in the Hydrogen isocyanide molecule ($\zeta=0.90$).
Analogously, Hydrogen atoms exhibit very high scaling factors in Oximes ($\zeta \approx 1.15$), where Oxygen and Nitrogen are present and in Hydrogen isocyanide, where the Hydrogen atom (unlike the Carbon atom) is very electron-poor ($\zeta = 1.16$).
Extensive benchmarking and future work on the connection between the local electron density and optimal basis function scaling factors, may help in finding even better descriptors or a parametrization for predicting $\boldsymbol{\zeta_\text{opt}}$.
Since this becomes increasingly complicated for larger basis sets, we believe that ML-based techniques nevertheless represent a suitable and computationally inexpensive solution to this problem.

\begin{figure*}[htb]
          \centering           
          \includegraphics[width=\linewidth]{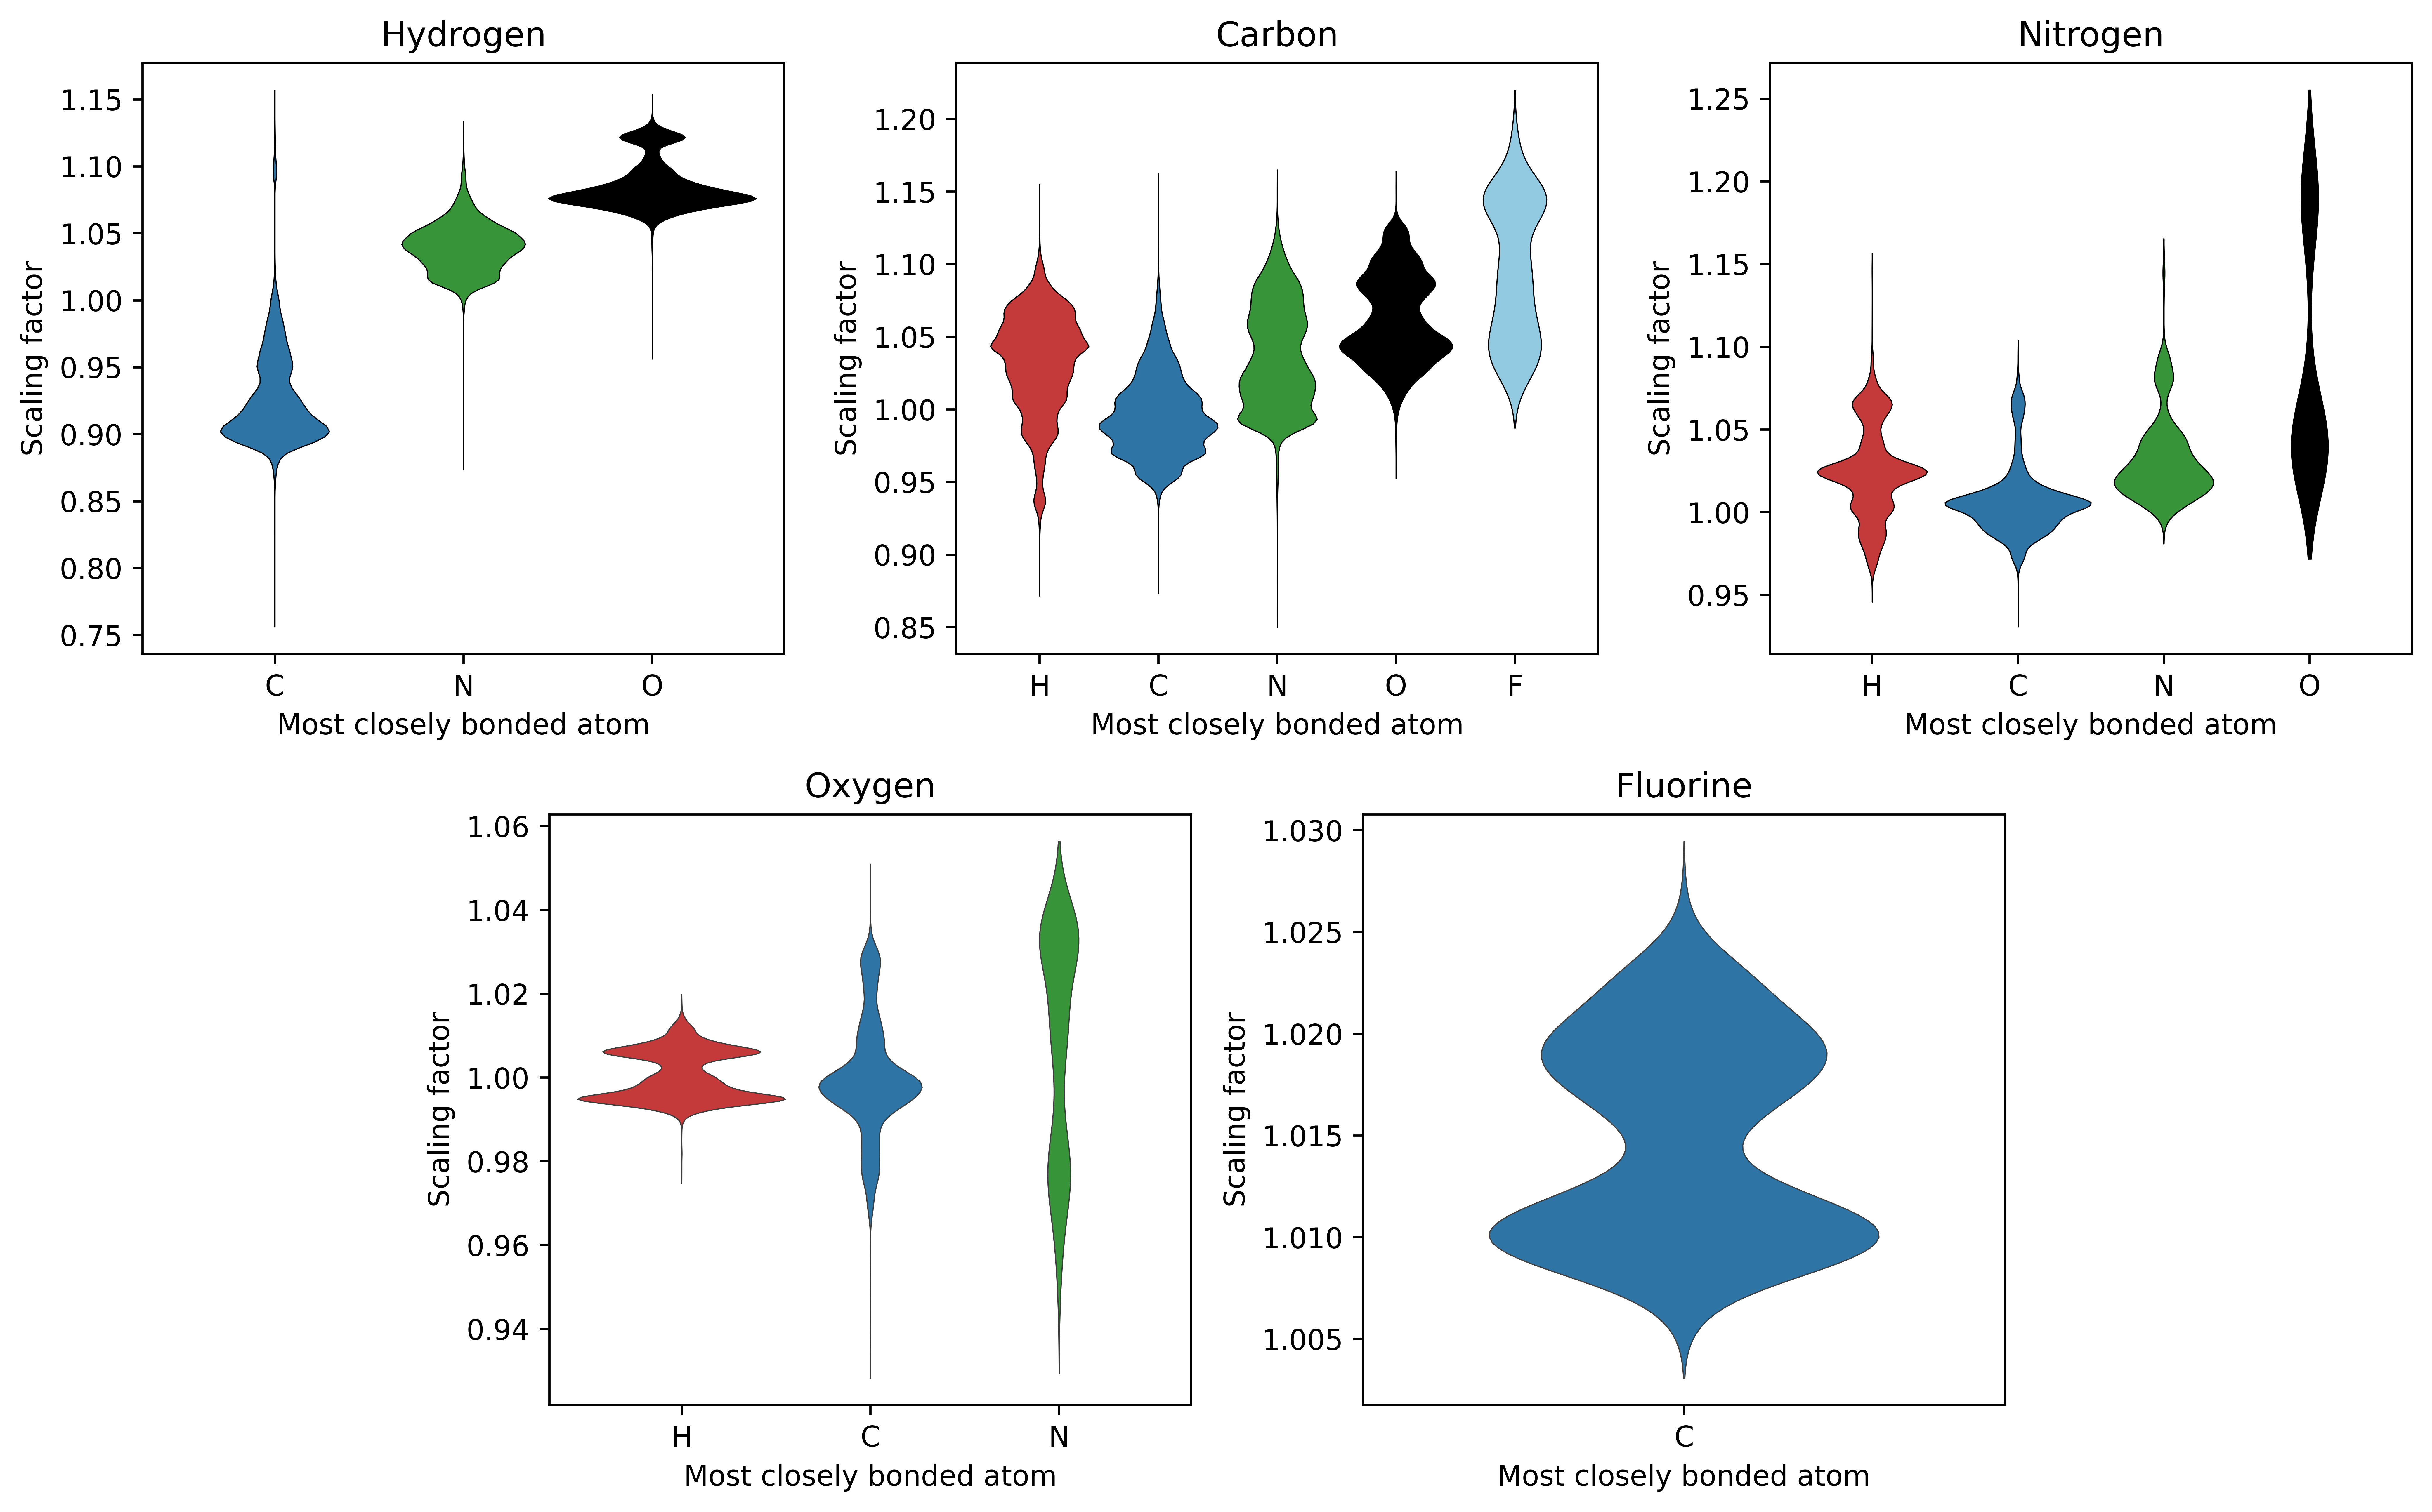}
          \caption{Element-wise STO-3G valence orbital scaling factor distributions sorted by closest bonding partner. 
%The position and number of lobes depend on the other atoms in the local environment, however can typically not be assigned to any single many diverse local chemical environments and a 
          Electronegative elements generally lead to larger scaling factors, which corresponds to a contraction of the Gaussian basis functions.}
    \label{fig:Violins}
 \end{figure*}

\begin{table*}[htbp]
    \centering
    \scalebox{0.8}{
    \hspace{-3.5mm}
    
    \begin{tabular}{|l|cccc|}
        \hline
         & \multicolumn{4}{c|}{\textbf{ Total energy change (kcal/mol)}} \\
         \hline
         \textbf{Molecule}\hspace{3mm} & \hspace{1mm}\textbf{aSTO-3G}\hspace{1mm}  &  \hspace{3mm}\textbf{a3-21G}\hspace{3mm} & \hspace{3mm}\textbf{a6-31G}\hspace{3mm} & \hspace{1mm}\textbf{a6-31G*}\hspace{3mm} \\
        \hline
        Aspirin & -9.74 & -54.3 & -5.20 & -2.16 \\
        % \hline
        Glucose & -2.38 & -57.3 & -3.27 & -3.16\\
        % \hline
         MDMA & -9.65 & -73.9 & -4.81 & -2.08\\
        % \hline
        Mescaline & -8.64 & -74.9 & -2.57 & +0.07\\
        % \hline
        Metformin & -16.3 & -37.0 & -2.52 & +6.53\\
        % \hline
        Methylglyoxal conf 1\, & -4.94 &  -19.8 & -1.61 & -1.87 \\
        % \hline
        Methylglyoxal conf 2\, & -4.96 & -21.1 & -1.89 & -2.25 \\ % 6-31G* improvement larger than 6-31G lol
        % \hline
        Nicotine & -11.2 & -58.9 & -1.91 & -1.21\\
        % \hline
         Paracetamol & -9.21 & -44.4 & -2.09 & -2.55 \\
        % \hline
        Resveratrol & -6.64 & -63.2 & -2.06 & -1.16\\
        % \hline
         Salicylic acid & -6.17 & -35.0 & -2.88 & -2.10 \\
        % \hline
        Uric acid & -25.0 & -40.9 & -5.83 & +3.93 \\
        \hline
    \end{tabular}
    }
    \caption{Hartree-Fock total energy change for biologicall/societally relevant molecules using adaptive vs default Pople-style basis sets. The larger prediction error in $\zeta$ for polarization functions (cf. Sec. \ref{sec:Results}) is reflected in selective energy increases using a6-31G*.}
    \label{tab:special_molecs_total_E}
\end{table*}
\begin{table*}[htbp]
    \centering
    \scalebox{0.8}{
    \hspace{-3.5mm}
    
    \begin{tabular}{|l|cccc|}
        \hline
         & \multicolumn{4}{c|}{\textbf{ Total energy change (kcal/mol)}} \\
         \hline
         \textbf{Molecule}\hspace{3mm} & \hspace{1mm}\textbf{aSTO-3G}\hspace{1mm}  &  \hspace{3mm}\textbf{a3-21G}\hspace{3mm} & \hspace{3mm}\textbf{a6-31G}\hspace{3mm} & \hspace{1mm}\textbf{a6-31G*}\hspace{3mm} \\
        \hline
        Aspirin & -9.74 & -54.3 & -5.20 & -2.16 \\
        % \hline
        Glucose & -2.38 & -57.3 & -3.27 & -3.16\\
        % \hline
         MDMA & -9.65 & -73.9 & -4.81 & -2.08\\
        % \hline
        Mescaline & -8.64 & -74.9 & -2.57 & +0.07\\
        % \hline
        Metformin & -16.3 & -37.0 & -2.52 & +6.53\\
        % \hline
        Methylglyoxal conf 1\, & -4.94 &  -19.8 & -1.61 & -1.87 \\
        % \hline
        Methylglyoxal conf 2\, & -4.96 & -21.1 & -1.89 & -2.25 \\ % 6-31G* improvement larger than 6-31G lol
        % \hline
        Nicotine & -11.2 & -58.9 & -1.91 & -1.21\\
        % \hline
         Paracetamol & -9.21 & -44.4 & -2.09 & -2.55 \\
        % \hline
        Resveratrol & -6.64 & -63.2 & -2.06 & -1.16\\
        % \hline
         Salicylic acid & -6.17 & -35.0 & -2.88 & -2.10 \\
        % \hline
        Uric acid & -25.0 & -40.9 & -5.83 & +3.93 \\
        \hline
    \end{tabular}
    }
    \caption{Hartree-Fock total energy change for biologicall/societally relevant molecules using adaptive vs default Pople-style basis sets. The larger prediction error in $\zeta$ for polarization functions (cf. Sec. \ref{sec:Results}) is reflected in selective energy increases using a6-31G*.}
    \label{tab:special_molecs_total_E}
\end{table*}
